# Supplementary material for: PARIC: Probabilistic Attention Regularization for Language Guided Image Classification from Pre-trained Vison Language Models
Source: arXiv:2503.11360 source file (2025-03-14)
Supplement: Supplementary file 1 [file 8_appendix.tex]

% Not needed as we were able to fit everything in 8 pages
\section{Appendix}
\label{sec:appendix}

\begin{figure}[h]
\centering
\includegraphics[scale=0.3]{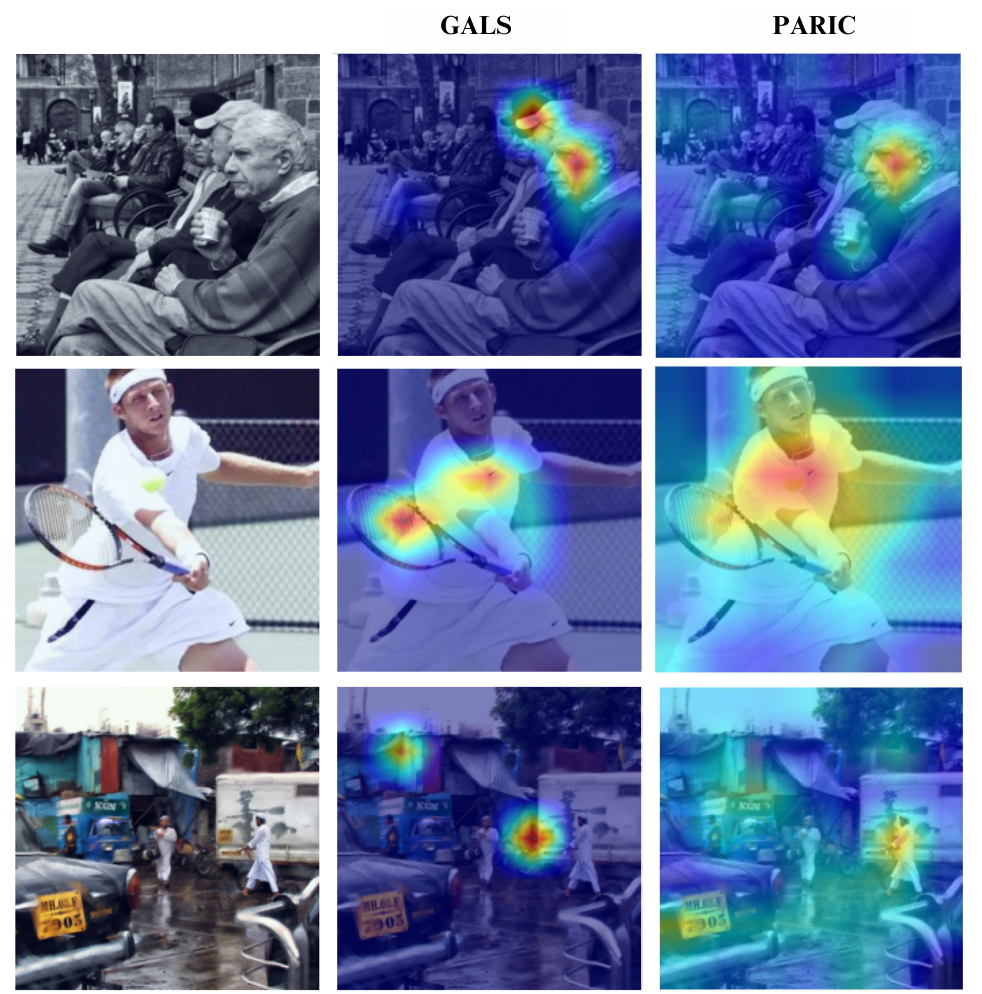}
\caption{\textbf{\textit{Attention maps for MSCOCO.}} Examples of effective attention maps for several instances from the MSCOCO dataset. In each row, the first image represents the original input, followed by the attention map from the frozen CLIP model. The third image shows the attention map obtained after integrating probabilistic layers and sampling 50 embedding using the mean aggregation method. }
\label{attmaps}
\end{figure}

\begin{figure}
% \centering
\includegraphics[scale=0.3]{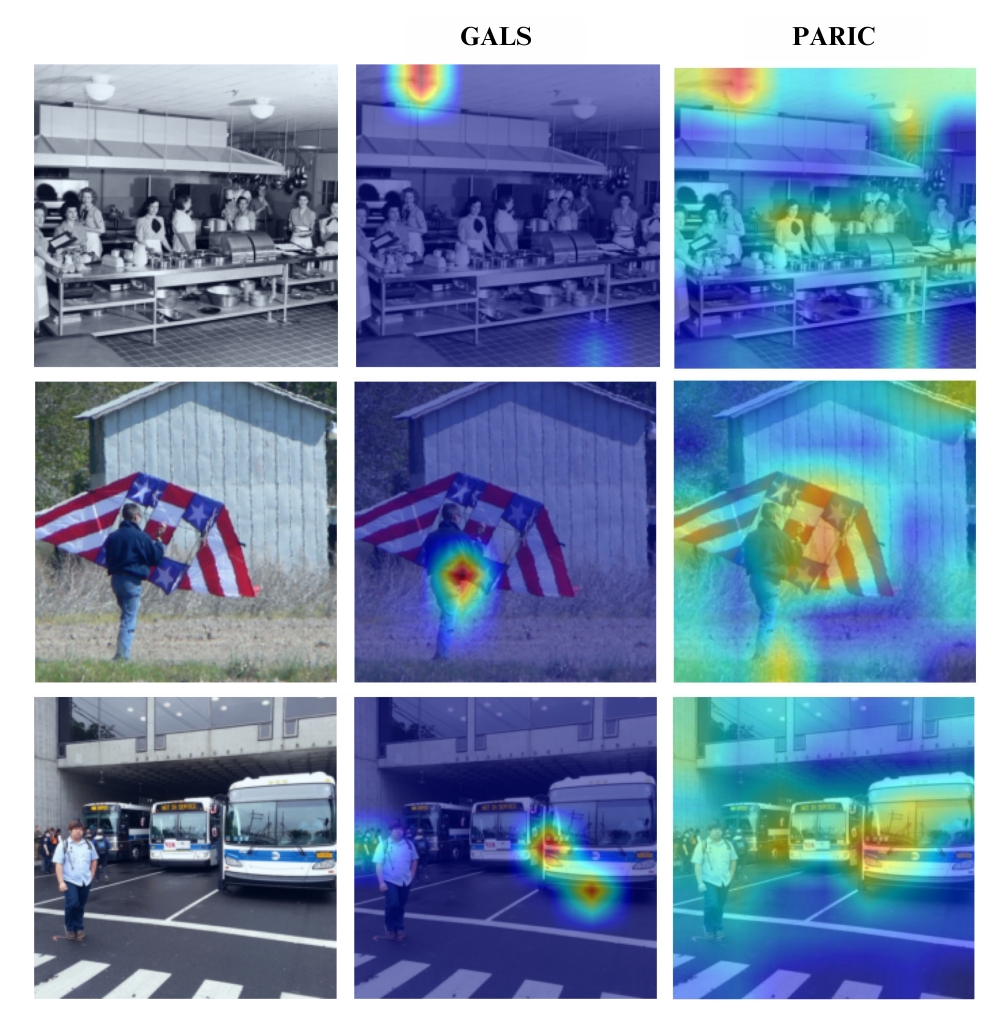}
\caption{\textbf{\textit{Poor Attention maps for MSCOCO.}} Examples of ineffective attention maps for several instances from the MSCOCO dataset. In each row, the first image represents the original input, followed by the attention map from the frozen CLIP model. The third image shows the attention map obtained after integrating probabilistic layers and sampling 50 embeddings using the mean aggregation method. }
\label{attmaps}
\end{figure}
